# Supplementary material for: IterativeCUR: Large Rank-Adaptive Approximation From a Small Recycled Sketch
Source: arXiv:2509.21963 source file (2026-09-22)
Supplement: Supplementary file 1 [file appendix.tex]

We now provide more numerical results demonstrating the performance of IterativeCUR across a reater array of problems. \cref{tab:test-matrices} contains a list of all matrices used in these experiments.
\begin{center}
    \begin{longtable}{|c|c|c|c|p{.27\linewidth}|}
        \caption{Description of matrices used in the experiments.} \label{tab:test-matrices} \\
        \hline
        Matrix & Matrix Size & Threshold & Exactly Low-Rank & Desciption \\ \hline
        Bayer01 & 57,735 &$5\times10^{-4}$ &False & Is a sparse unsymmetric matrix from SuiteSparse library. The matrix arises from chemical simulation. \\  \hline
        Bcircuit & 68,902 &$1\times10^{-1}$ &False & Is a $7 \times 10^{-5}$-sparse unsymetric matrix from the SuiteSparse library. Matrix arises form circuit simulations.\\ \hline
         C-67 & 57,975 & $1\times10^{-2}$&False & Is a sparse symmetric matrix coming from the SuiteSparse library. Matrix arises from optimization problems.\\ \hline
        C-69 & 67,458 &$2\times10^{-3}$ &False & Is a $1 \times 10^{-4}$sparse symmetric matrix from the SuiteSparse library. Matrix arises from optimization problems.\\  \hline
        Cauchy & 30,000 & $1\times10^{-5}$& 20 &Is a dense symmetric matrix with entries defined by $\frac{1}{i+j}$.\\  \hline
        Ct20Stif & 52,329 &$7\times10^{-4}$ & False & Is a  $9 \times 10^{-4}$-sparse symmetric matrix from the SuiteSparse library. Matrix is a stiffness matrix for a ct20 engine block.\\  \hline
        G7Jac200 & 59,310 & & False & Is a $2 \times 10^{-4}$-sparse unsymmetric matrix from the SuiteSparse library. Matrix arises from optimization problems.\\   \hline
        Hilbert & 30,000 &$1\times10^{-5}$ &20 & Is a dense symmetric matrix with entries defined by $\frac{1}{i+j-1}$.\\  \hline
        Low-Rank & 30,000 &$1\times10^{-6}$ &2,000 &  Generate two Gaussian matrices $G_i \in \mathbb{R}^{30,000 \times 2,000}$, $i \in \{1,2\}$. Then set $A = G_1G_2^\top$.\\  \hline
         Low-Rank PD& 30,000 & $2\times10^{-2}$& False & Generate two Gaussian matrices $G_i \in \mathbb{R}^{30,000 \times 2,000}, i \in \{1,2\}$. Then set $A = G_1G_2^\top + \text{Diag}((1-\exp(\frac{\log(30,000)}{\log(5)})^{1:20,000})$.\\ \hline
         Mark3 & 64,089 &$5\times10^{-2}$ & False & Is a $9 \times 10^{-5}$-sparse unsymmetric matrix from the SuiteSparse library. Matrix arises from economics problems.\\  \hline
        RandLOW & 70,000 &$5\times10^{-3}$ & 4,000 &Generate two Gaussian matrices $G_i \in \mathbb{R}^{70,000 \times 4,000}$, $i \in \{1,2\}$. Then generate $D=\text{Diag}(1/1:4000)$ and set $A = G_1 DG_2^\top$. \\ \hline
         RandSVD & 30,000 &$5\times10^{-3}$ & False & Generated from the gallery function in Matlab. The condition number is specified as $1 \times 10^{16}$ with geometrically decaying singular values.\\ \hline
        TSOPF & 76,216 & $1\times10^{-1}$& False & Is a $3 \times 10^{-4}$-sparse symmetric matrix from the SuiteSparse library. Matrix arises form power network problems.\\ \hline
        Venkat01 & 62,424 & $1\times10^{-1}$& False & Is a $4 \times 10^{-4}$-sparse unsymmetric matrix from the SuiteSparse library. Matrix arises from fluid dynamics sequence.\\  \hline
    \end{longtable} 
\end{center}


\section{Continuation of Threshold Experiments}
Here we include the remaining results from the threshold experiments described in \cref{subsec:threshold}. In some of these examples we observe IterativeCUR achieving a worse accuracy than the other approaches. It should be noted that in those examples, the rank of the approximation of IterativeCUR is much lower than the other approaches and the accuracy achieved is below the threshold.
\begin{figure}[H]
    \centering
    \input{./plots/synthetic_comparisons/bayer01_57735_250_0.tex}
    \caption{Box plots for the performance of  SVDSketch (SVDs), s-LUPP, and Iterative LUPP applied to a Bayer01 matrix generated according to \cref{tab:test-matrices}.}
    \label{fig:bayer01}
\end{figure}
\begin{figure}[H]
    \centering
    \input{./plots/synthetic_comparisons/c-69_67458_250_0.tex}
    \caption{Box plots for the performance of  SVDSketch (SVDs), s-LUPP, and Iterative LUPP applied to a C-69 matrix generated according to \cref{tab:test-matrices}.}
    \label{fig:c-69}
\end{figure}
\begin{figure}[H]
    \centering
    \input{./plots/synthetic_comparisons/c-67_57975_250_0.tex}
    \caption{Box plots for the performance of  SVDSketch (SVDs), s-LUPP, and Iterative LUPP applied to a C-67 matrix generated according to \cref{tab:test-matrices}.}
    \label{fig:c-67}
\end{figure}
\begin{figure}[H]
    \centering
    \input{./plots/synthetic_comparisons/ct20stif_52329_250_0.tex}
    \caption{Box plots for the performance of  SVDSketch (SVDs), s-LUPP, and Iterative LUPP applied to a Ct20Stif matrix generated according to \cref{tab:test-matrices}.}
    \label{fig:ct20stif}
\end{figure}
\begin{figure}[H]
    \centering
    \input{./plots/synthetic_comparisons/cauchy_30000_10_0.tex}
    \caption{Box plots for the performance of  SVDSketch (SVDs), s-LUPP, and Iterative LUPP applied to a Cauchy matrix generated according to \cref{tab:test-matrices}.}
    \label{fig:cauchy}
\end{figure}
\begin{figure}[H]
    \centering
    \input{./plots/synthetic_comparisons/hilbert_30000_10_0.tex}
    \caption{Box plots for the performance of  SVDSketch (SVDs), s-LUPP, and Iterative LUPP applied to  a Hilbert matrix generated according to  \cref{tab:test-matrices}.}
    \label{fig:hilbert}
\end{figure}

\begin{figure}[H]
    \centering
    \input{./plots/synthetic_comparisons/low_rank_pd_30000_250_0.tex}
    \caption{Box plots for the performance of  SVDSketch (SVDs), s-LUPP, and Iterative LUPP applied to a low-rank matrix plus decaying diagonal matrix generated according to  \cref{tab:test-matrices}.}
    \label{fig:low_rank_pd_comp}
\end{figure}
\begin{figure}[H]
    \centering
    \input{./plots/synthetic_comparisons/mark3_64089_250_0.tex}
    \caption{Box plots for the performance of  SVDSketch (SVDs), s-LUPP, and Iterative LUPP applied to a Mark3 matrix generated according to \cref{tab:test-matrices}.}
    \label{fig:mark3}
\end{figure}
\begin{figure}[H]
   \centering
   \input{./plots/synthetic_comparisons/g7jac200_59310_250_0.tex}
   \caption{Box plots for the performance of  SVDSketch (SVDs), s-LUPP, and Iterative LUPP applied to a G7Jac200 matrix generated according to \cref{tab:test-matrices}.}
   \label{fig:g7jac}
\end{figure}
\begin{figure}[H]
    \centering
    \input{./plots/synthetic_comparisons/randLOW_70000_250_0.tex}
    \caption{Box plots for the performance of  SVDSketch (SVDs), s-LUPP, and Iterative LUPP applied to a RandLOW matrix generated according to \cref{tab:test-matrices}.}
    \label{fig:randLOW}
\end{figure}
\begin{figure}[H]
    \centering
    \input{./plots/synthetic_comparisons/randsvd_30000_250_0.tex}
    \caption{Box plots for the performance of  SVDSketch (SVDs), s-LUPP, and Iterative LUPP applied to a rand svd matrix generated according to  \cref{tab:test-matrices}.}
    \label{fig:rand_svd_comp}
\end{figure}
\begin{figure}[H]
    \centering
    \input{./plots/synthetic_comparisons/tsopf_76216_250_0.tex}
    \caption{Box plots for the performance of  SVDSketch (SVDs), s-LUPP, and Iterative LUPP applied to a TSOPF matrix generated according to \cref{tab:test-matrices}.}
    \label{fig:tsopf}
\end{figure}
\begin{figure}[H]
    \centering
    \input{./plots/synthetic_comparisons/venkat01_62424_250_0.tex}
    \caption{Box plots for the performance of  SVDSketch (SVDs), s-LUPP, and Iterative LUPP applied to a Venkat01 matrix generated according to \cref{tab:test-matrices}.}
    \label{fig:venkat01}
\end{figure}

\section{Continuation of Fixed Rank Experiments}
Here we display the results for the remaining fixed rank experiments from \cref{subsec:fixed_rank}. In these experiments, we see the consistent story that IterativeCUR matches s-LUPP in accuracy and typically beats it in performance. In a few experiments, we see s-LUPP outperforms IterativeCUR in time, its possible that, because we were unable to completely control resource the usage by other jobs, these time differences are because of differences in resource use. 

\begin{figure}[H]
     \centering
     \input{./plots/same_rank/c-67_250_0.tex}
     \caption{This plot shows the change in approximation accuracy and computational time for \svds, \icurl, and \curs with approximations of varying rank.}
     \label{fig:fixed_rank_c-67}
 \end{figure}
\begin{figure}[H]
    \centering
    \input{./plots/same_rank/c-69_250_0.tex}
    \caption{This plot shows the change in approximation accuracy and computational time for \svds, \icurl, and \curs with approximations of varying rank.}
    \label{fig:fixed_rank_c-69}
\end{figure}
\begin{figure}[H]
    \centering
    \input{./plots/same_rank/ct20stif_250_0.tex}
    \caption{This plot shows the change in approximation accuracy and computational time for \svds, \icurl, and \curs with approximations of varying rank.}
    \label{fig:fixed_rank_ct20stif}
\end{figure}

\begin{figure}[H]
    \centering
    \input{./plots/same_rank/mark3_250_0.tex}
    \caption{This plot shows the change in approximation accuracy and computational time for \svds, \icurl, and \curs with approximations of varying rank.}
    \label{fig:fixed_rank_mark3}
\end{figure}
\begin{figure}[H]
    \centering
    \input{./plots/same_rank/tsopf_250_0.tex}
    \caption{This plot shows the change in approximation accuracy and computational time for \svds, \icurl, and \curs with approximations of varying rank.}
    \label{fig:fixed_rank_tsopf}
\end{figure}

\begin{figure}[H]
    \centering
    \input{./plots/same_rank/bcircuit_250_0.tex}
    \caption{This plot shows the change in approximation accuracy and computational time for \svds, \icurl, and \curs with approximations of varying rank.}
    \label{fig:fixed_rank_bcircuit}
\end{figure}

\begin{figure}[H]
    \centering
    \input{./plots/same_rank/randlow_250_0.tex}
    \caption{This plot shows the change in approximation accuracy and computational time for \svds, \icurl, and \curs with approximations of varying rank.}
    \label{fig:fixed_rank_randlow}
\end{figure}
\begin{figure}[H]
    \centering
    \input{./plots/same_rank/randsvd_250_0.tex}
     \caption{This plot shows the change in approximation accuracy and computational time for \svds, \icurl, and \curs with approximations of varying rank.}
    \label{fig:fixed_rank_randsvd}
\end{figure}
\begin{figure}[H]
    \centering
    \input{./plots/same_rank/venkat01_250_0.tex}
    \caption{This plot shows the change in approximation accuracy and computational time for \svds, \icurl, and \curs with approximations of varying rank.}
    \label{fig:fixed_rank_venkat}
\end{figure}

\section{The Kahan Matrix}
It is also interesting to consider the performance of ItertaiveCUR on known difficult examples such as the Kahan matrix. This set of experiments considers in-depth the performance on these examples.

\begin{figure}
    \centering
    \input{./plots/kahan/kahan_median_acc.tex}
    \caption{Comparison of time and accuracy of IterativeCUR for block sizes 5, 50, 100, and 500 for a Low-Rank PD matrix generated according to \cref{tab:test-matrices}.}
    \label{fig:kahan-acc}
\end{figure}
\begin{figure}
    \centering
    \input{./plots/kahan/kahan_var_acc.tex}
    \caption{Comparison of time and accuracy of IterativeCUR for block sizes 5, 50, 100, and 500 for a Low-Rank PD matrix generated according to \cref{tab:test-matrices}.}
    \label{fig:kahan-var-acc}
\end{figure}
